# Supplementary material for: Miniature work-to-work converter engine powered by motor protein
Source: arXiv:2503.07112 source file (2025-12-03)
Supplement: Supplementary file 1 [file Supplementary.pdf]

# Feedback controlled microengine powered by motor protein

Suraj Deshmukh,<sup>1</sup> Basudha Roy,<sup>1</sup> Sougata Guha,<sup>2</sup> Shivprasad Patil,<sup>3</sup> Arnab Saha,<sup>4</sup> and Sudipto Muhuri<sup>5,1,\*</sup>

<sup>1</sup>*Department of Physics, Savitribai Phule Pune University, Pune 411007, India*

<sup>2</sup>*INFN Napoli, Complesso Universitario di Monte S. Angelo, Napoli 80126, Italy*

<sup>3</sup>*Department of Physics, Indian Institute of Science Education and Research, Pune 411008, India*

<sup>4</sup>*Department of Physics, University Of Calcutta, Kolkata 700009, India*

<sup>5</sup>*School of Physics, University of Hyderabad, Hyderabad 500046, India*

Supplementary Information

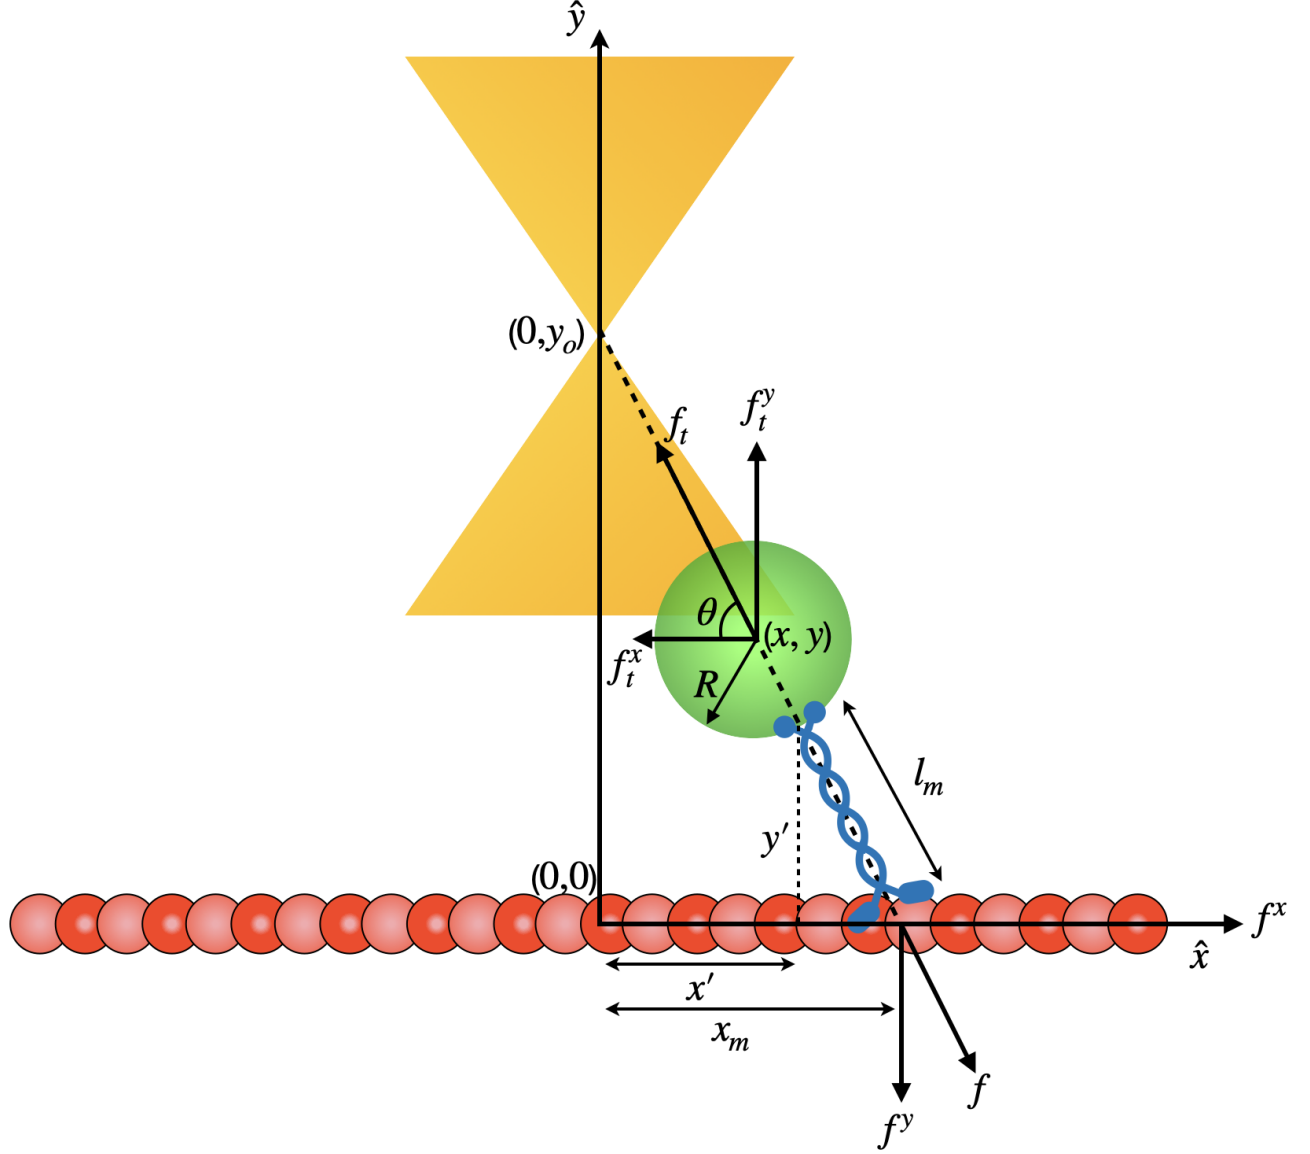

Fig. S1. 2D schematic of the force-balanced condition for cargo transported by a single motor under optical trap. The cargo bead has a radius of length  $R$  and is moving in  $\hat{x} - \hat{y}$  plane. The MT is assumed to be along  $\hat{x}$  direction. The optical trap center is positioned at  $(0, y)$  while the cargo position is denoted by  $(x, y)$ . The motor is attached to the MT at  $(x_m, 0)$  and makes an angle  $\theta$  with the MT. As the motor walks along the MT both  $x_m$  and  $\theta$  changes. The other end of the motor is attached to the cargo and the position of the contact between cargo and the motor is denoted as  $(x', y')$ . The cargo is experiencing two forces - force due to motor extension ( $f$ ) and trap force ( $f_t$ ). The components of these two forces along  $x$  and  $y$ -directions are denoted as  $f^x$ ,  $f^y$ ,  $f_t^x$  and  $f_t^y$  respectively.

## TWO DIMENSIONAL STOCHASTIC ANALYSIS OF CARGO TRANSPORT

### Force-balance conditions

Similar to the one-dimensional analysis, the motor in this case is modeled as a harmonic spring with a spring constant  $k_m$ . As the motor progresses along the underlying MT filament, it exerts a pulling force on the bead. This force is counteracted by the restoring force arising from the optical trap's harmonic potential. Both the forces acting on the bead and its displacement vector from the center of the optical trap typically have components in two

directions: the horizontal direction, aligned with the MT axis, and the vertical direction, perpendicular to it (Fig. S1).

For simplicity, we assume the microtubule (MT) lies along the X-axis at  $y_{MT} = 0$ , with the optical trap center located at  $(0, y_o)$ . Here,  $y_o$  is defined as  $y_o = l_o + R$ , where  $l_o$  represents the rest length of the motor, and  $R$  is the radius of the bead (cargo). At  $t = 0$ , we assume the motor is attached to the MT, and the bead is positioned at the trap center. Consequently, at  $t = 0$ , the motor is vertically aligned at  $x_m = 0$ , and its length equals its rest length ( $l_o$ ).

As the motor progresses along the microtubule (MT), it stretches beyond its rest length, generating a restoring force that acts on the cargo in the direction of the motor's extension. This restoring force causes the cargo to deviate from the trap center, thereby activating the optical trap force, which pulls the cargo back toward the trap center. The equilibrium position of the cargo and the orientation of the motor - characterized by the angle  $\theta$  formed between the motor head and the MT - are determined by the balance between these opposing forces and the torques they produce. The resulting torques cause the cargo to rotate about its center, reaching equilibrium when the motor aligns along the line connecting the cargo center to the trap center. Under these conditions, the force balance can be expressed as,

$$k_t^x x = k_m \Theta(l_m - l_o) \left[ (x_m - x') - l_o \frac{(x' - x)}{R} \right] \quad (1)$$

$$k_t^y (y_o - y) = k_m \Theta(l_m - l_o) \left[ y' - l_o \frac{(y - y')}{R} \right] \quad (2)$$

where  $x_m$  is the motor position on the MT,  $l_m$  is the length of the motor,  $(x', y')$  is the motor binding position on the cargo surface and  $(x, y)$  is the position of the cargo center,  $\Theta$  is the Heavy-side theta function,  $k_t^x$  and  $k_t^y$  are the trap stiffness along horizontal and vertical directions, respectively (Fig. S1) [1]. In this study, we have always taken  $k_t^y = k_t^x/3$  [2, 3].

It is important to note that the force balance condition between the motor force and the trap force in the vertical direction (Eq. 2) remains valid only as long as the cargo does not come into contact with the underlying MT. Once the motor progresses along the MT and the bead makes contact with the MT, an additional normal force (acting in the vertical direction) will act on the bead [4–6]. In such a scenario, the vertical force balance will be determined by this normal force in addition to the trap force and the motor force in the vertical direction. Consequently, when the cargo touches the MT, only the horizontal force balance condition (Eq. 1) should be considered.

From a geometric perspective, the motor binding position  $(x', y')$  must satisfy the following equation:

$$(x' - x)^2 + (y' - y)^2 = R^2 \quad (3)$$

Therefore at equilibrium,

$$\tan \theta = \frac{y'}{x_m - x'} = \frac{y}{x_m - x} \quad (4)$$

By simultaneously solving these four equations, the steady state of the system (values of  $x, y, x', y'$ ) can be determined for a given motor position  $x_m$ .

### Stochastic simulation of motor dynamics

We use force-balance conditions and geometric constraints (Eqs. 1, 2, 3 and 4) to perform stochastic simulations of single dynein-driven cargo transport under an optical trap. As time progresses, the motor head, attached to the MT, moves away from its initial position while experiencing the trap force. The force ( $f$ ) acting on the motor at any moment is given by  $f = k_m(l_m - l_o)$ , where  $l_m > l_o$  and  $l_m = \sqrt{(x_m - x)^2 + y^2}$ . The motor's velocity under load follows the relationship  $v_m = v_o(1 - f/f_s)$ , where  $v_o$  is the motor's velocity without load, and  $f_s$  is its stall force.

During each simulation step of duration  $\Delta t$ , the motor either detaches from the MT at an unbinding rate  $\varepsilon$  (Eq. 5 from the main text) or attempts to take a step of size  $d$  with a probability  $P(\Delta t) = v_m \Delta t / d$ . In this study, we chose  $\Delta t = 10^{-4} s$  and  $d = 8 nm$  [7]. After each step, the force-balance conditions are recalculated to update the values

of  $x$ ,  $y$ ,  $x'$ , and  $y'$  based on Eqs. 1, 2, 3, and 4. The simulation terminates when the motor detaches from the MT, and the corresponding time is recorded as the First Passage Time. All properties are averaged over  $10^5$  independent simulation runs.

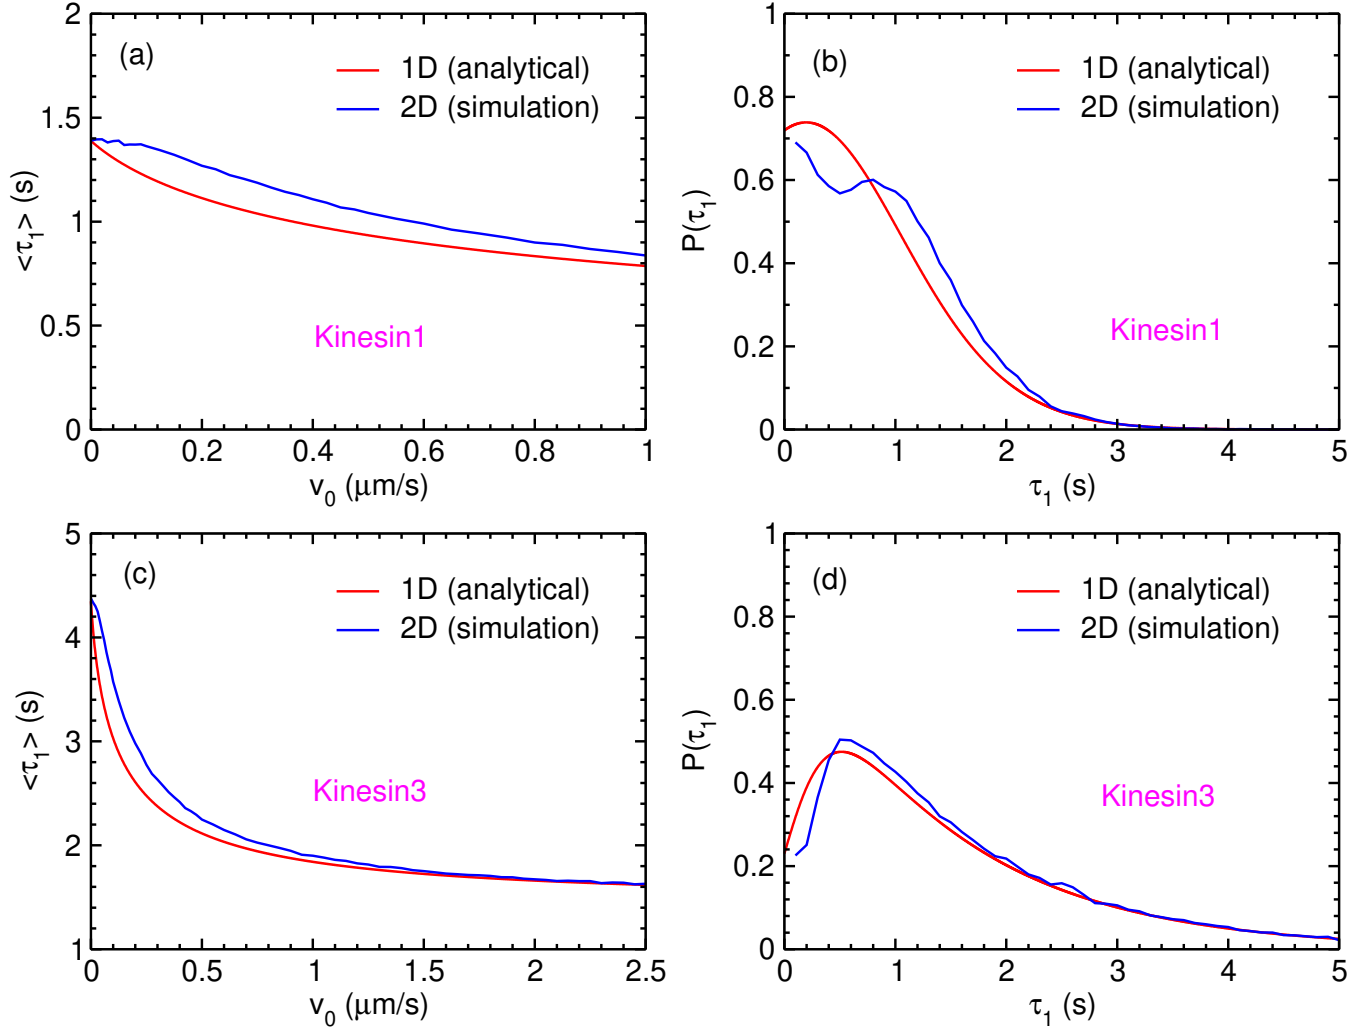

Fig. S2. Comparison of 2D stochastic simulations with 1D analytical form for  $k_t^x = 0.005 \text{ pN/nm}$ : (a) Variation of Average run time of *kinesin-1* motor ( $\tau_1$ ) with  $v_o$ , (b) Probability distribution of run time for *kinesin-1* motor when  $v_o = 0.8 \mu\text{m/s}$ , (c) Variation of Average run time of *kinesin-3* motor ( $\tau_1$ ) with  $v_o$ , (d) Probability distribution of run time for *kinesin-3* motor when  $v_o = 2.3 \mu\text{m/s}$ . 2D Stochastic simulation is done for a disc of radius  $0.5 \mu\text{m}$  and restlength of kinesin motor  $l_o = 110 \text{ nm}$ .

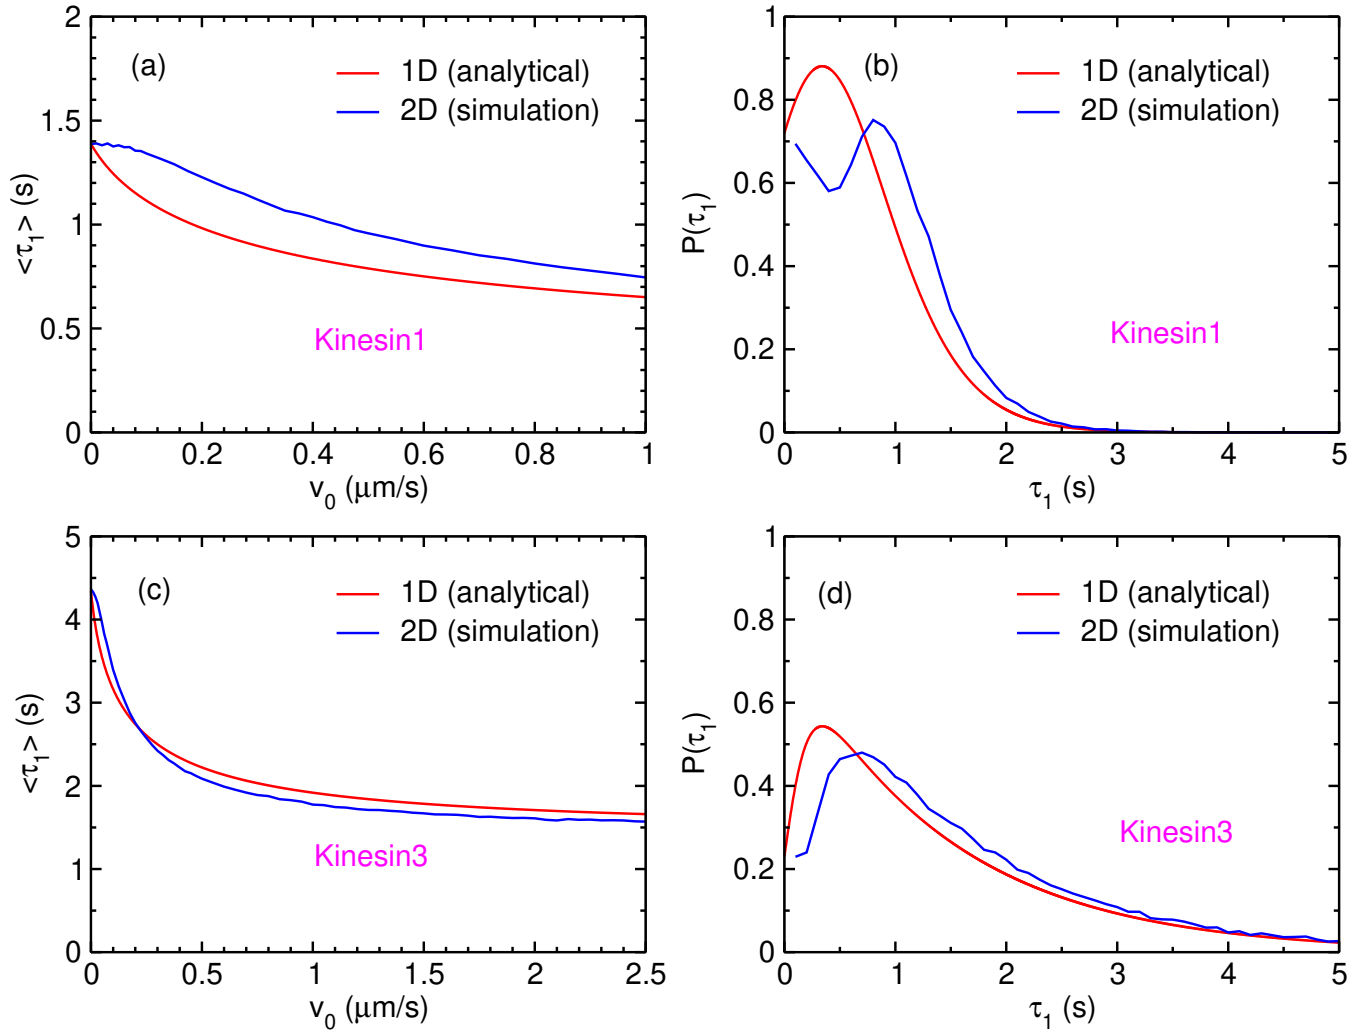

Fig. S3. Comparison of 2D stochastic simulations with 1D analytical form for  $k_t^x = 0.01 \text{ pN/nm}$ : (a) Variation of Average run time of *kinesin-1* motor ( $\tau_1$ ) with  $v_o$ , (b) Probability distribution of run time for *kinesin-1* motor when  $v_o = 0.8 \mu\text{m/s}$ , (c) Variation of Average run time of *kinesin-3* motor ( $\tau_1$ ) with  $v_o$ , (d) Probability distribution of run time for *kinesin-3* motor when  $v_o = 2.3 \mu\text{m/s}$ . 2D Stochastic simulation is done for a disc of radius  $0.5 \mu\text{m}$  and restlength of kinesin motor  $l_o = 110 \text{ nm}$ .

\* sudiptomuhuri@uoh.ac.in

- [1] Naren Sundararajan, Sougata Guha, Sudipto Muhuri, and Mithun K Mitra. Theoretical analysis of cargo transport by catch bonded motors in optical trapping assays. *Soft Matter*, 20(3):566–577, 2024.
- [2] Arthur Ashkin. Forces of a single-beam gradient laser trap on a dielectric sphere in the ray optics regime. *Biophysical journal*, 61(2):569–582, 1992.
- [3] Volker Bormuth, Anita Jannasch, Marcel Ander, Carlos M van Kats, Alfons van Blaaderen, Jonathon Howard, and Erik Schäffer. Optical trapping of coated microspheres. *Optics express*, 16(18):13831–13844, 2008.
- [4] Michael E Fisher and Young C Kim. Kinesin crouches to sprint but resists pushing. *Proceedings of the National Academy of Sciences*, 102(45):16209–16214, 2005.
- [5] Hamid Khataee and Jonathon Howard. Force generated by two kinesin motors depends on the load direction and inter-molecular coupling. *Physical review letters*, 122(18):188101, 2019.
- [6] Serapion Pyrpasopoulos, Henry Shuman, and E Michael Ostap. Modulation of kinesin's load-bearing capacity by force geometry and the microtubule track. *Biophysical journal*, 118(1):243–253, 2020.
- [7] Mark J Schnitzer and Steven M Block. Kinesin hydrolyses one atp per 8-nm step. *Nature*, 388(6640):386–390, 1997.
